# Supplementary material for: Leverage Score Sampling for Faster Accelerated Regression and ERM
Source: arXiv:1711.08426 source file (2017-11-22)
Supplement: Supplementary file 1 [file Appendix.tex]

%!TEX root = arxiv.tex
\section{Computing Leverage Scores given a Regression Algorithm}
\label{sec:computeleveragescores}
In this section we give a proof of Lemma \ref{lem:computing_leverage_scores} which bounds the running time of computing leverage scores assuming access to a regression algorithm. The main algorithm is given as Algorithm \ref{alg:computeLS}.

\begin{proof}[Proof of Lemma~\ref{lem:computing_leverage_scores}]
	Let $y_{j}^{*}=(\ma^{\top}\ma)^{-1}\ma^{\top}v_{j}$ be the minimizer of
	$f_{\ma,v_{j}}(x)$. (\ref{eq:dist_guarantee}) shows that
	\[
	\norm{\ma y_{j}-\ma y_{j}^{*}}_{2}^{2}\leq\epsilon\cdot v_{j}^{\top}\ma(\ma^{\top}\ma)^{-1}\ma^{\top}v_{j}.
	\]
	Using $v_{j}\sim N(0,I)$, we have that
\[
v_{j}^{\top}\ma(\ma^{\top}\ma)^{-1}\ma^{\top}v_{j}\leq2d\cdot\log(n)
\]
	with probability $1-n^{-\Theta(1)}$. Hence, we have that
	\[
	\left|e_{i}^{\top}\ma y_{j}-e_{i}^{\top}\ma y_{j}^{*}\right|\leq\norm{\ma y_{j}-\ma y_{j}^{*}}_{2}\leq\sqrt{2\epsilon d\cdot\log(n)}.
	\]
	Using this and 
\begin{equation*}
\left|e_{i}^{\top}\ma y_{j}^{*}\right| \leq \sqrt{e_{i}^{\top}\ma(\ma^{\top}\ma)^{-1}\ma^{\top}e_{i}}\sqrt{v_{j}^{\top}\ma(\ma^{\top}\ma)^{-1}\ma^{\top}v_{j}} \leq\sqrt{2d\cdot\log(n)} ~,
\end{equation*}
	we have that
	\[
	\left|\left(e_{i}^{\top}\ma y_{j}\right)^{2}-\left(e_{i}^{\top}\ma y_{j}^{*}\right)^{2}\right|\leq6\sqrt{\epsilon}d\cdot\log(n).
	\]
	Using the definition of $\epsilon$, we have that
	\begin{equation}
	\left|\frac{1}{k}\sum_{j=1}^{k}(e_{i}^{\top}\ma y_{j})^{2}-\frac{1}{k}\sum_{j=1}^{k}(e_{i}^{\top}\ma y_{j}^{*})^{2}\right| \leq 6\sqrt{\epsilon}d\cdot\log(n)\leq\frac{\delta}{3n\cdot\kappa(\ma^{\top}\ma)}\label{eq:JL_err}
	\end{equation}
	Also, we note that
	\[
	\frac{1}{k}\sum_{j=1}^{k}(e_{i}^{\top}\ma y_{j}^{*})^{2}=\frac{1}{k}\sum_{j=1}^{k}(e_{i}^{\top}\ma (\ma^{\top}\ma)^{-1}\ma^{\top}v_{j})^{2}.
	\]
	Since $v_{j}\sim N(0,I)$ and $k=c\log(n)/\delta^{2}$ where $c$
	is some large enough constant, Johnson-Lindenstrauss lemma
	shows that, with high probability in $n$ for all $i \in [n]$
	\[
	\left(1-\frac{\delta}{3}\right)\sigma_{i}(\ma)\leq\frac{1}{k}\sum_{j=1}^{k}(e_{i}^{\top}\ma y_{j}^{*})^{2}
	\leq \left(1+\frac{\delta}{3}\right)\sigma_{i}(\ma)
	\]
	Combining this with (\ref{eq:JL_err}) gives the result.
	
	Finally, to check the success probability of this algorithm, we note
	that we solved $O(\delta^{-2}\log n)$ many regression problems and
	each one has success probability $1-n^{-\Theta(1)}$. Also, the Johnson\textendash Lindenstrauss
	lemma succeed with probability $1-n^{-\Theta(1)}$. This gives the
	result.
\end{proof}

\section{Reductions between High Probability and Expected Running Time}
\label{sec:proofreductionlemma}
\subsection{Proof of Lemma \ref{lemma:reduction}}
\begin{proof}[Proof of Lemma \ref{lemma:reduction}]
	To show the lemma we will show the existence of a procedure (described in Algorithm \ref{alg:mainalgoreduction}) which produces a point $x'$ such that 
	\begin{equation}
	\label{eqn:genintermed1}
		F(x') - F(x^*) \leq 1/2 \left(F(x_0) - F(x^*) \right)
	\end{equation}
	with expected running time bounded by $O\left((\runtime + \runtime')\log(r)\right)$. Applying this procedure $O(\log(\epsilon^{-1})$ and using linearity of expectation gives us the Lemma \ref{lemma:reduction}. 
	Consider the following procedure to prove Lemma \ref{lemma:reduction}.
	\begin{algorithm2e}[h]
	
	\caption{$\mathtt{Reduction}(x_{0},F(x),\mathcal{P},\alg, c, \delta, r)$}
	
	\label{alg:mainalgoreduction}
	
	\SetAlgoLined
	Set $T = \log_{c^{-1}}(2r^2)$

	\Repeat{$E \leq 0.5$}{
		\For{$i = 0 \rightarrow T$}{
			\For{$j = 0 \rightarrow \log_{\delta^{-1}}(2 \log_{c^{-1}}(2r^2)$}{
				Set $x_{ij} = \alg(x_i, F)$
			}
			Set $x_{i+1} = \min_{j} x_{ij}$
		}
		Compute error estimates $E_1 = \mathcal{P}(x_0), E_2 = \mathcal{P}(x_T)$

		Set $E = \frac{E_2}{E_1}$. 
	}
	\textbf{Output:} $x_T$
	
\end{algorithm2e}

Note that since for every $x_{ij}$ we have that 
\[F(x_{ij}) - F(x^*) \leq c \left( F(x_i) - F(x^*) \right)\]
with probability at least $\delta$, therefore we have that 
\[F(x_{i+1}) - F(x^*) \leq c \left( F(x_{i}) - F(x^*) \right)\]
with probability at least $1 - \delta^{\log_{\delta^{-1}}(2 \log_{c^{-1}}(r^2)} = 1 - \frac{1}{2 \log_{c^{-1}}(r^2)}$. Taking a union bound over the outer loop gives us that with probability at least $1/2$ we have that 
\[F(x_{T}) - F(x^*) \leq \frac{1}{2r^2} \left( F(x_{i}) - F(x^*) \right)\] 
Moreover by the property of the estimates given by $\mathcal{P}$ we know that in this case we have that $E \leq 0.5$. Therefore we have that with probability at least $1/2$ the repeat loop computes an $x_T$ that reduces error by at least a factor of $1/2$ and we can verify it. Therefore in expectation the loop runs a total of $2$ times. 
The total runtime of the above procedure can easily seen to be
$O\left((\runtime + \runtime')\log(r)\log(\epsilon^{-1}\right)$.

Further suppose we are given a procedure with the guarantee that for any $\epsilon$ in expected running time $\runtime_{\epsilon}$ it produces a point $x'$ such that 
\[F(x') - \min F(x) \leq \epsilon(F(x_0) - \min F(x))\]
We now run this procedure for time $\runtime_{\epsilon/2}$. By Markov's inequality with probability at least $1/2$ we have a point that satisfies 
\[F(x') - \min F(x) \leq \epsilon(F(x_0) - \min F(x))\]
It is now easy to see that if we repeat the above procedure $\log(\gamma^{-1})$ many times and take the $x$ with the minimum value we have a point $x'$ such that 
\[F(x') - \min F(x) \leq \epsilon(F(x_0) - \min F(x))\]
with probability at least $1 - \gamma$.
\end{proof}

\section{Proofs and Theorems from the Generalized ERM Section}
\label{sec:gen_erm:proofs}

\subsection{Accelerated Coordinate Descent for ERM}
\label{sec:accproof}
\begin{proof}[Proof of Theorem~\ref{thm:standard_solvers_gen_ERM}]
	To remind the reader
\[
f(x)=\sum_{i=1}^{n}\psi_{i}(a_{i}^{\top}x)
\text{ where }\psi_{i}''(x)\in [\mu_i, L_i] ~.
\]
Following is a well known theorem. For a proof see \cite{kakade2009applications}. 
\begin{thm}[Strong / Smooth Duality] A closed and convex function $f$ is $\beta$-strongly convex with respect to a norm $\| \cdot \|$ if and only if $f^*$ is $\frac{1}{\beta}$-strongly smooth w.r.t the dual norm of $\| \cdot \|$.   
\end{thm}
A direct application of the above theorem gives us that $\psi_{i}^{*''}(y) \in [\frac{1}{L_i}, \frac{1}{\mu_i}]$. Consider the function
	\begin{equation*}
	g_{s}(y) =\sum_{i=1}^{n}\psi_{i}^{*}(y_{i})+\frac{1}{2\lambda}\norm{\ma^{\top}y}_{2}^{2}-s^{\top}\ma^{\top}y
	\end{equation*}
	Consider the following modified function $\tilde{g}_s(y) \defeq g_s(\md y)$ where $\md$ is a diagonal matrix with $\md_{ii} = L_i$. We will equivalently minimize the function $\tilde{g}_s(y_i)$. We now immediately get that the function $\tilde{g}_s(y)$ is $1$ strongly convex. Moreover we have that
	\[
	\frac{d^{2}}{dy_{i}^{2}}g_{s}(y)= \frac{L_i}{\mu_i} + \frac{1}{\lambda}\norm{a_{i}}^{2}L_i~.
	\]
	Hence, Theorem~\ref{thm:corr_desc} finds $y$ satisfying \eqref{eq:dual_req}	in time
\begin{equation*}
O\left(s(\ma) \cdot\sum_{i \in [n]}\sqrt{\frac{L_i}{\mu_i}+\frac{1}{\lambda}\norm{a_{i}}^{2}L_i}\log(\epsilon^{-1})\right)
= O \left(\left(\sum_{i=1}^{n} \sqrt{\frac{L_i}{\mu_i}} + \frac{1}{\sqrt{\lambda}}\sum_{i=1}^{n}\|a_i\|\sqrt{L_i}\right)s(\ma)\log(\epsilon^{-1}) \right)
\end{equation*}
	A direct application of Theorem \ref{thm:proxpoint} gives that the total running time is
	\[ O \left(\left(\sum_{i=1}^{n} \sqrt{\frac{L_i}{\mu_i}} + \frac{1}{\sqrt{\lambda}}\sum_{i=1}^{n}\|a_i\|\sqrt{L_i}\right)s(\ma) \log(n \kappa) \log(\kappa / \epsilon) \right)
	\]
The above equation assumes that the inner iterations of accelerated coordinate descent can be implemented in $O(s(\ma))$. This is easy to see because diagonal scaling is linear in sparsity. Therefore the only bottleneck is computing the gradient of the dual function $\psi^*$. We can assume that $\psi$ is explicit and therefore the gradient of $\psi^*$ is easily computed.
\end{proof}

\subsection{A Matrix Concentration Inequality for Sampling with Replacement}
\label{sec:concentrationinequality}
\begin{lem}
\label{lemma:concwithreplacement}
	Given an error parameter $0 \leq \epsilon \leq 1$, let $u$ be a vector of leverage score overestimates, i.e. $\sigma_i(\ma) \leq u_i$ for all $i$. Let $\alpha = \epsilon^{-2}$ be a sampling rate parameter and $c$ be a fixed constant. For each row we define a number $\gamma_i = \min\{1, \alpha c u_i \log(d)\}$ and a probability $p_i = \frac{\gamma_i}{\sum \gamma_i}$. Let $Y_j$ be a random variable which is sampled by picking a vector $a_i$ with probability $p_i$ and setting $Y_j = \frac{a_ia_i^\top}{p_i}$. Now consider the random variable $Y = \frac{1}{m} \sum_j Y_j$. We have that
	as long as $m \geq \sum_i \gamma_i$ then
	\[ \Pr( (1 - \epsilon)\ma^\top\ma \preceq Y \preceq (1 + \epsilon) \ma^\top \ma) \geq 1 - d^{-c/3}\] 
\end{lem}
\begin{proof}
	The proof of the lemma follows the proof of Lemma 4 in \cite{uniformSampling}. We only state the differences. We use the inequality given in \cite{harvey2012matrix}.

	\begin{lem}
	\label{lemma:tropplemma}
		Let $Y_1 \ldots Y_k$ be independent random positive semidefinite matrices of size $d \times d$. Let $Y = \sum Y_i$ and let $Z = \E[Y]$. If $Y_i \preceq R.Z$ then
		\[ \Pr \left[ \sum Y_i \preceq (1 - \epsilon)Z \right] \leq de^{-\frac{\epsilon^2}{2R}}
\enspace
	\text{ and }
\enspace
		 \Pr \left[ \sum Y_i \succeq (1 + \epsilon)Z \right] \leq de^{-\frac{\epsilon^2}{3R}} 
~.
\]
	\end{lem}

	Note that the expectation of $Y_j/m = a_i a_i^\top/m$. Moreover note that each 
	\[ \frac{Y_j}{m} \preceq \max_i \frac{a_i a_i^\top \sum_k \gamma_k}{m \gamma_i} \preceq \frac{\ma^\top \ma}{c \log d \epsilon^{-2}}\]
	The inequality follows from noting that $m \geq \sum \gamma_i$ and Equation 10 in \cite{uniformSampling}. The calculations now follow exactly in the same way as in the proof in \cite{uniformSampling}. 
\end{proof}
\subsection{Proof of Lemma \ref{lemma:SVRGLemma}}
\label{app:lemma:SVRG}

\begin{proof}[Proof of Lemma \ref{lemma:SVRGLemma}]
Let $x_* \defeq \argmin\;g(x)$. Define auxiliary functions 
\[h_i(x) \defeq g_i(x) - g_i(x_*) - \nabla g_i(x_*)^{\top}(x - x_*)\]
We know that $h_i(x_*) = \min h_i(x)$ since $\nabla h_i(x_*) = 0$. Using smoothness of $h$ and that $h_i(x_*) = 0$, we now have that 
\[ \|\nabla h_i(x)\|^2_2 \leq 2Lh_i(x)\]
A simple substitution gives us that for all $i$
\[ \|\nabla g_i(x) - \nabla g_i(x_*)\|^2_2 \leq 2L \left( g_i(x) - g_i(x_*) - \nabla g_i(x_*)^{\top}(x - x_*) \right)\]
Taking expectations and using the fact that $g(x_*) = 0$ gives us that 
\[\E_{i \sim D} \|\nabla g_i(x) - \nabla g_i(x_*)\|^2_2 \leq 2L(g(x) - g(x^*))\] 	
\end{proof}
